# Supplementary material for: Goodhart's Law in Reinforcement Learning
Source: arXiv:2310.09144 source file (2023-10-13)
Supplement: Supplementary file 1 [file goodharting_happens_appendix.tex]

\section{Goodharting runs}\label{appendix:environments}

With each set of parameters of a specific setting, we randomly perform experiments and average over their results. Specifically, we randomly pick a true reward function, and then for each distance $d$, we randomly select 10 proxy rewards that are $d$ away from the true reward. Then, we evaluate the agents trained on these proxy rewards, and average over their performances.
